# Supplementary material for: Modality Alignment Meets Federated Broadcasting
Source: arXiv:2411.15837 source file (2024-11-24)
Supplement: Supplementary file 1 [file appendix.tex]

% CVPR 2025 Paper Template; see https://github.com/cvpr-org/author-kit

\documentclass[10pt,twocolumn,letterpaper]{article}

%%%%%%%%% PAPER TYPE  - PLEASE UPDATE FOR FINAL VERSION
% \usepackage{cvpr}              % To produce the CAMERA-READY version
\usepackage[review]{cvpr}      % To produce the REVIEW version
\input{preamble}
\definecolor{cvprblue}{rgb}{0.21,0.49,0.74}
\usepackage[pagebackref,breaklinks,colorlinks,allcolors=cvprblue]{hyperref}
\usepackage{multirow}
\usepackage{colortbl}

%%%%%%%%% PAPER ID  - PLEASE UPDATE
 % *** Enter the Paper ID here

\begin{document}

{
\newpage
    \small
    \bibliographystyle{ieeenat_fullname}
    \bibliography{main}
}

{
\newpage
    \small
    \bibliographystyle{ieeenat_fullname}
    \bibliography{main}
}

\end{document}
